# Supplementary material for: Directional Variance Adjustment: improving covariance estimates for high-dimensional portfolio optimization
Source: arXiv:1109.3069 source file (2012-03-08)
Supplement: Supplementary file 1 [file appendix.tex]

%!TEX root = /Users/danielbartz/dbmlu/publications/papers/2012_01_DVA_revision2/JoCSaDA_DVA.tex
%%%%%%%%%%%%%%%%%%%%%%%%%%%%%%%%%%%%%%%%%%%%%%%%%%%%%%%%
In Figure~\ref{fig:USbv_reg},~\ref{fig:UScv_reg},~\ref{fig:EUbv_reg},~\ref{fig:EUcv_reg}~and~\ref{fig:HKv_reg}, realized (out-of-sample) portfolio variances for varying regularization strength $\lambda$ are shown for the market samples from the last section. Here, the performance measure is directly optimized. In this case, our proposed  method outperforms the other methods for all market samples, for

\begin{figure} 
\begin{center}
\includegraphics[width=.85\textwidth]{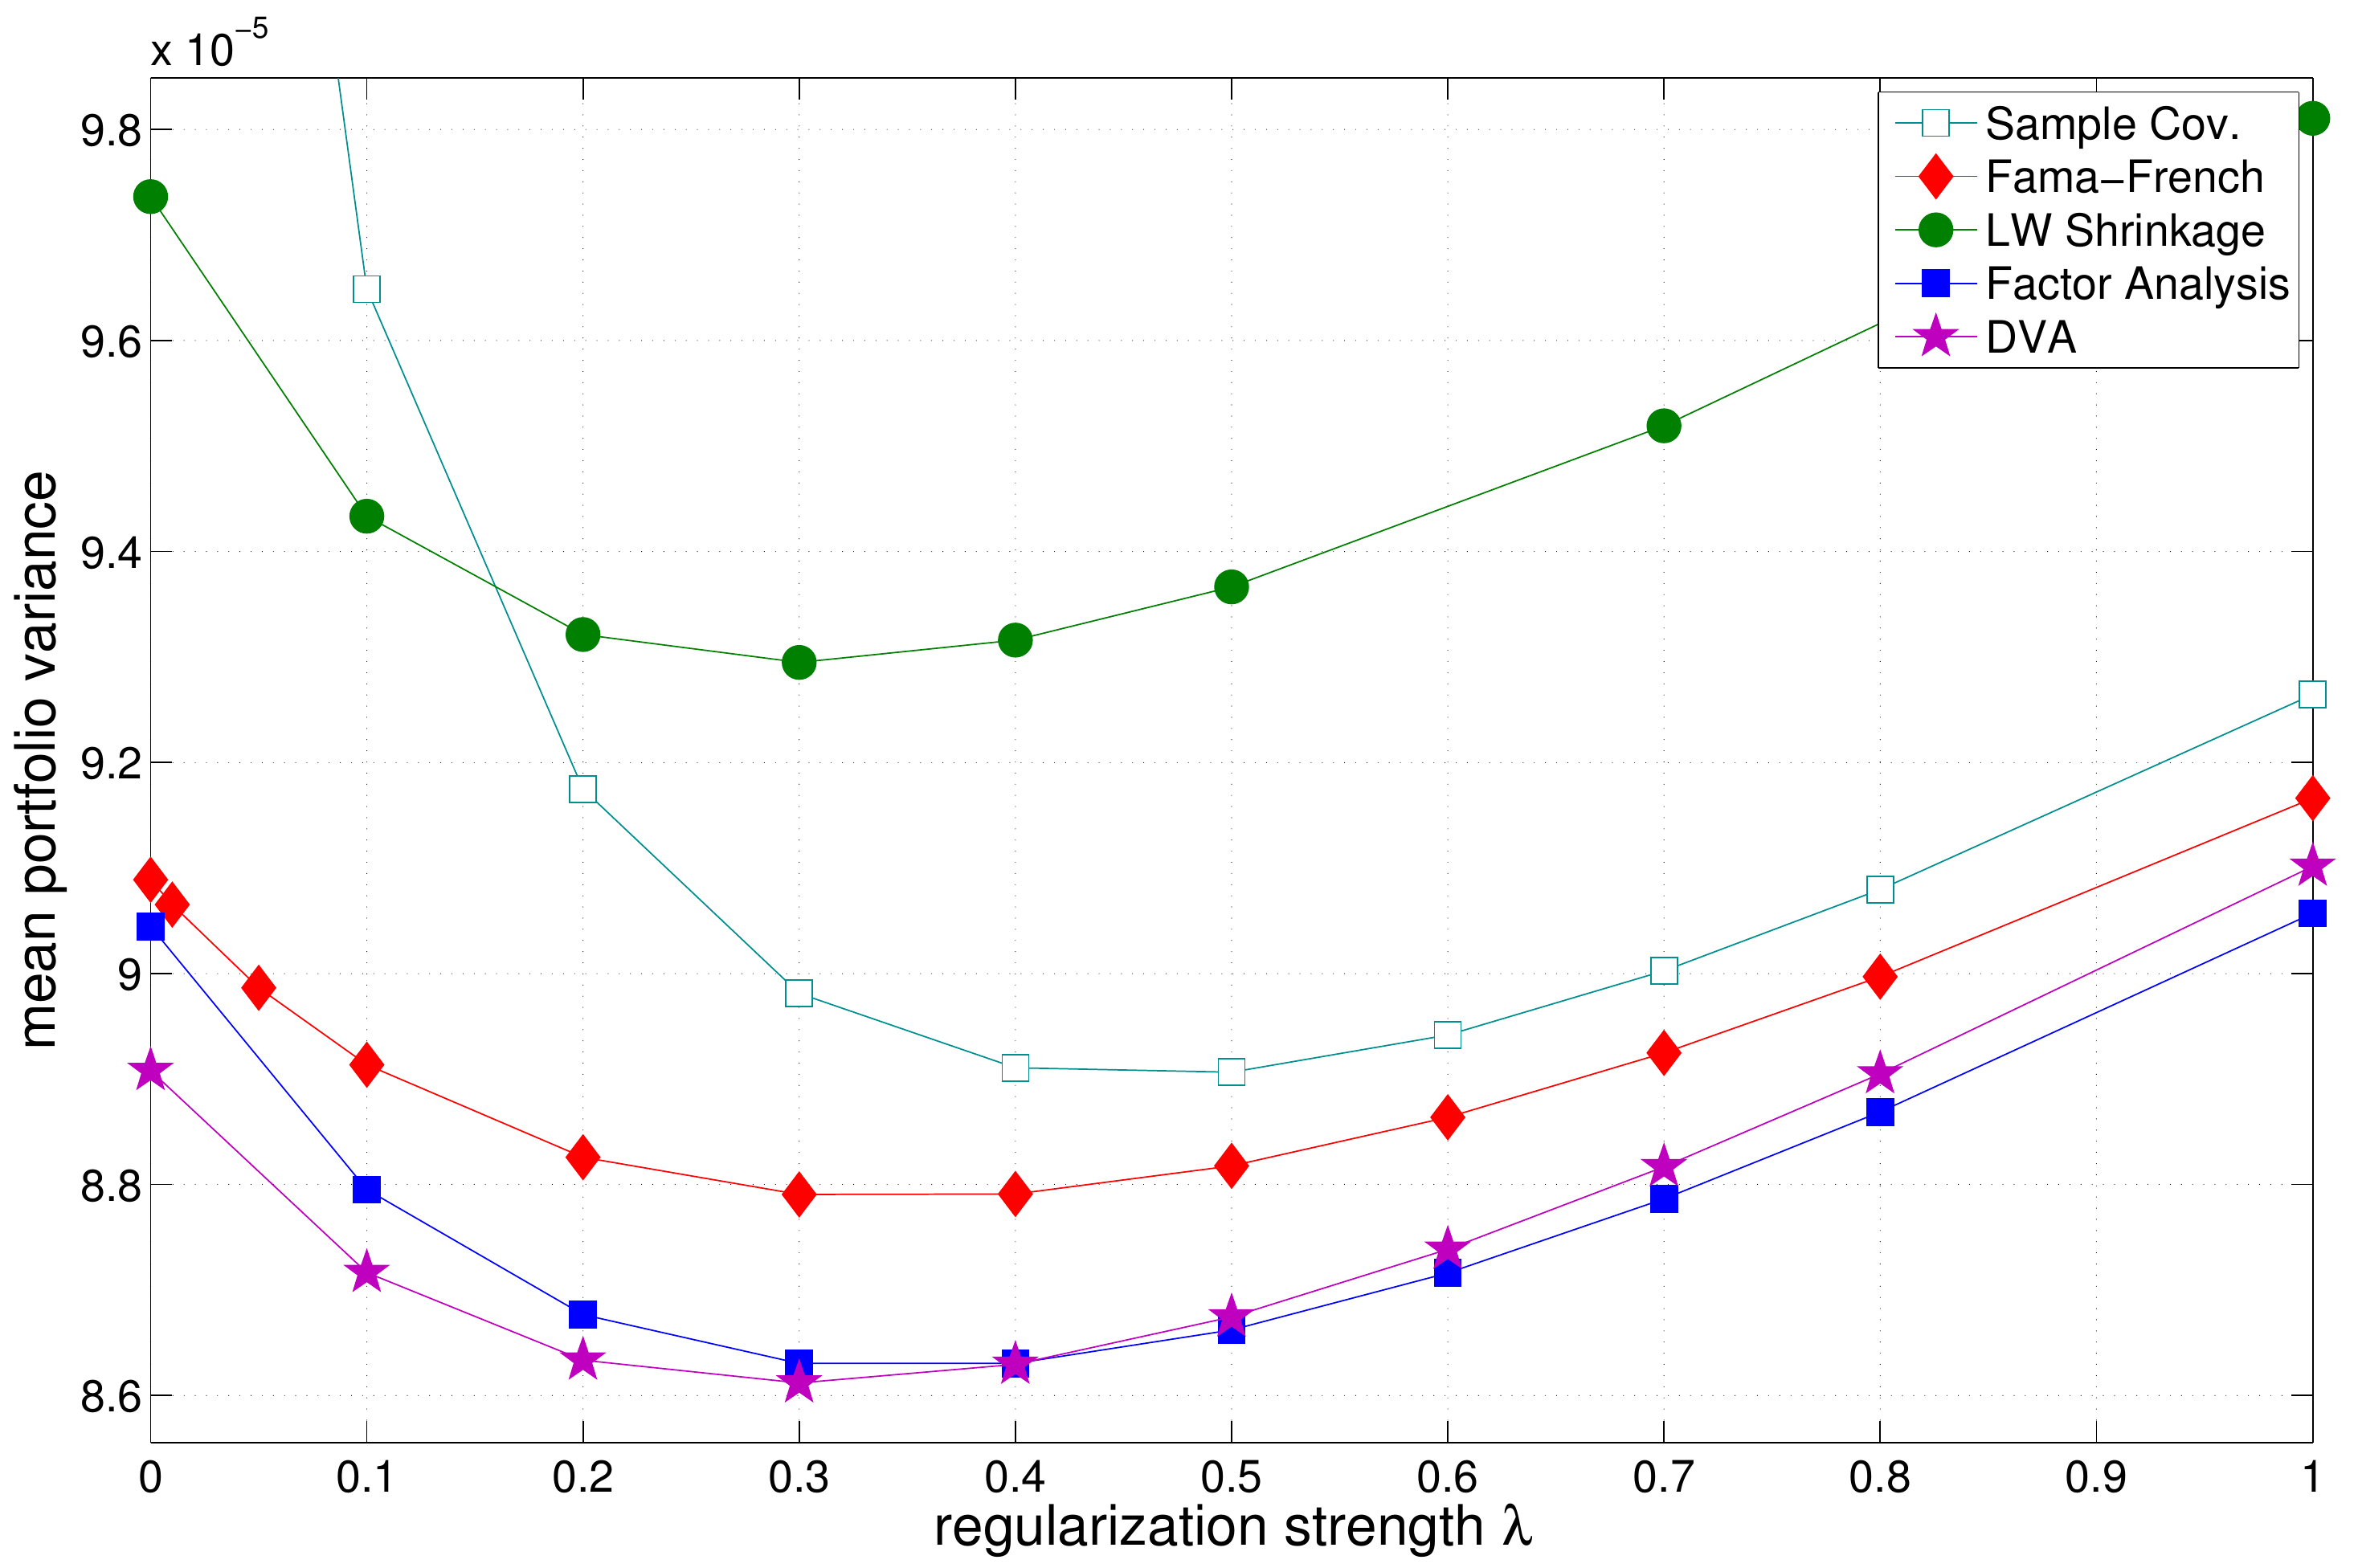}
\caption{variance of optimized portfolios. US market sample~a}
 \label{fig:USbv_reg}
\end{center}
\end{figure}

\begin{figure} 
\begin{center}
\includegraphics[width=.85\textwidth]{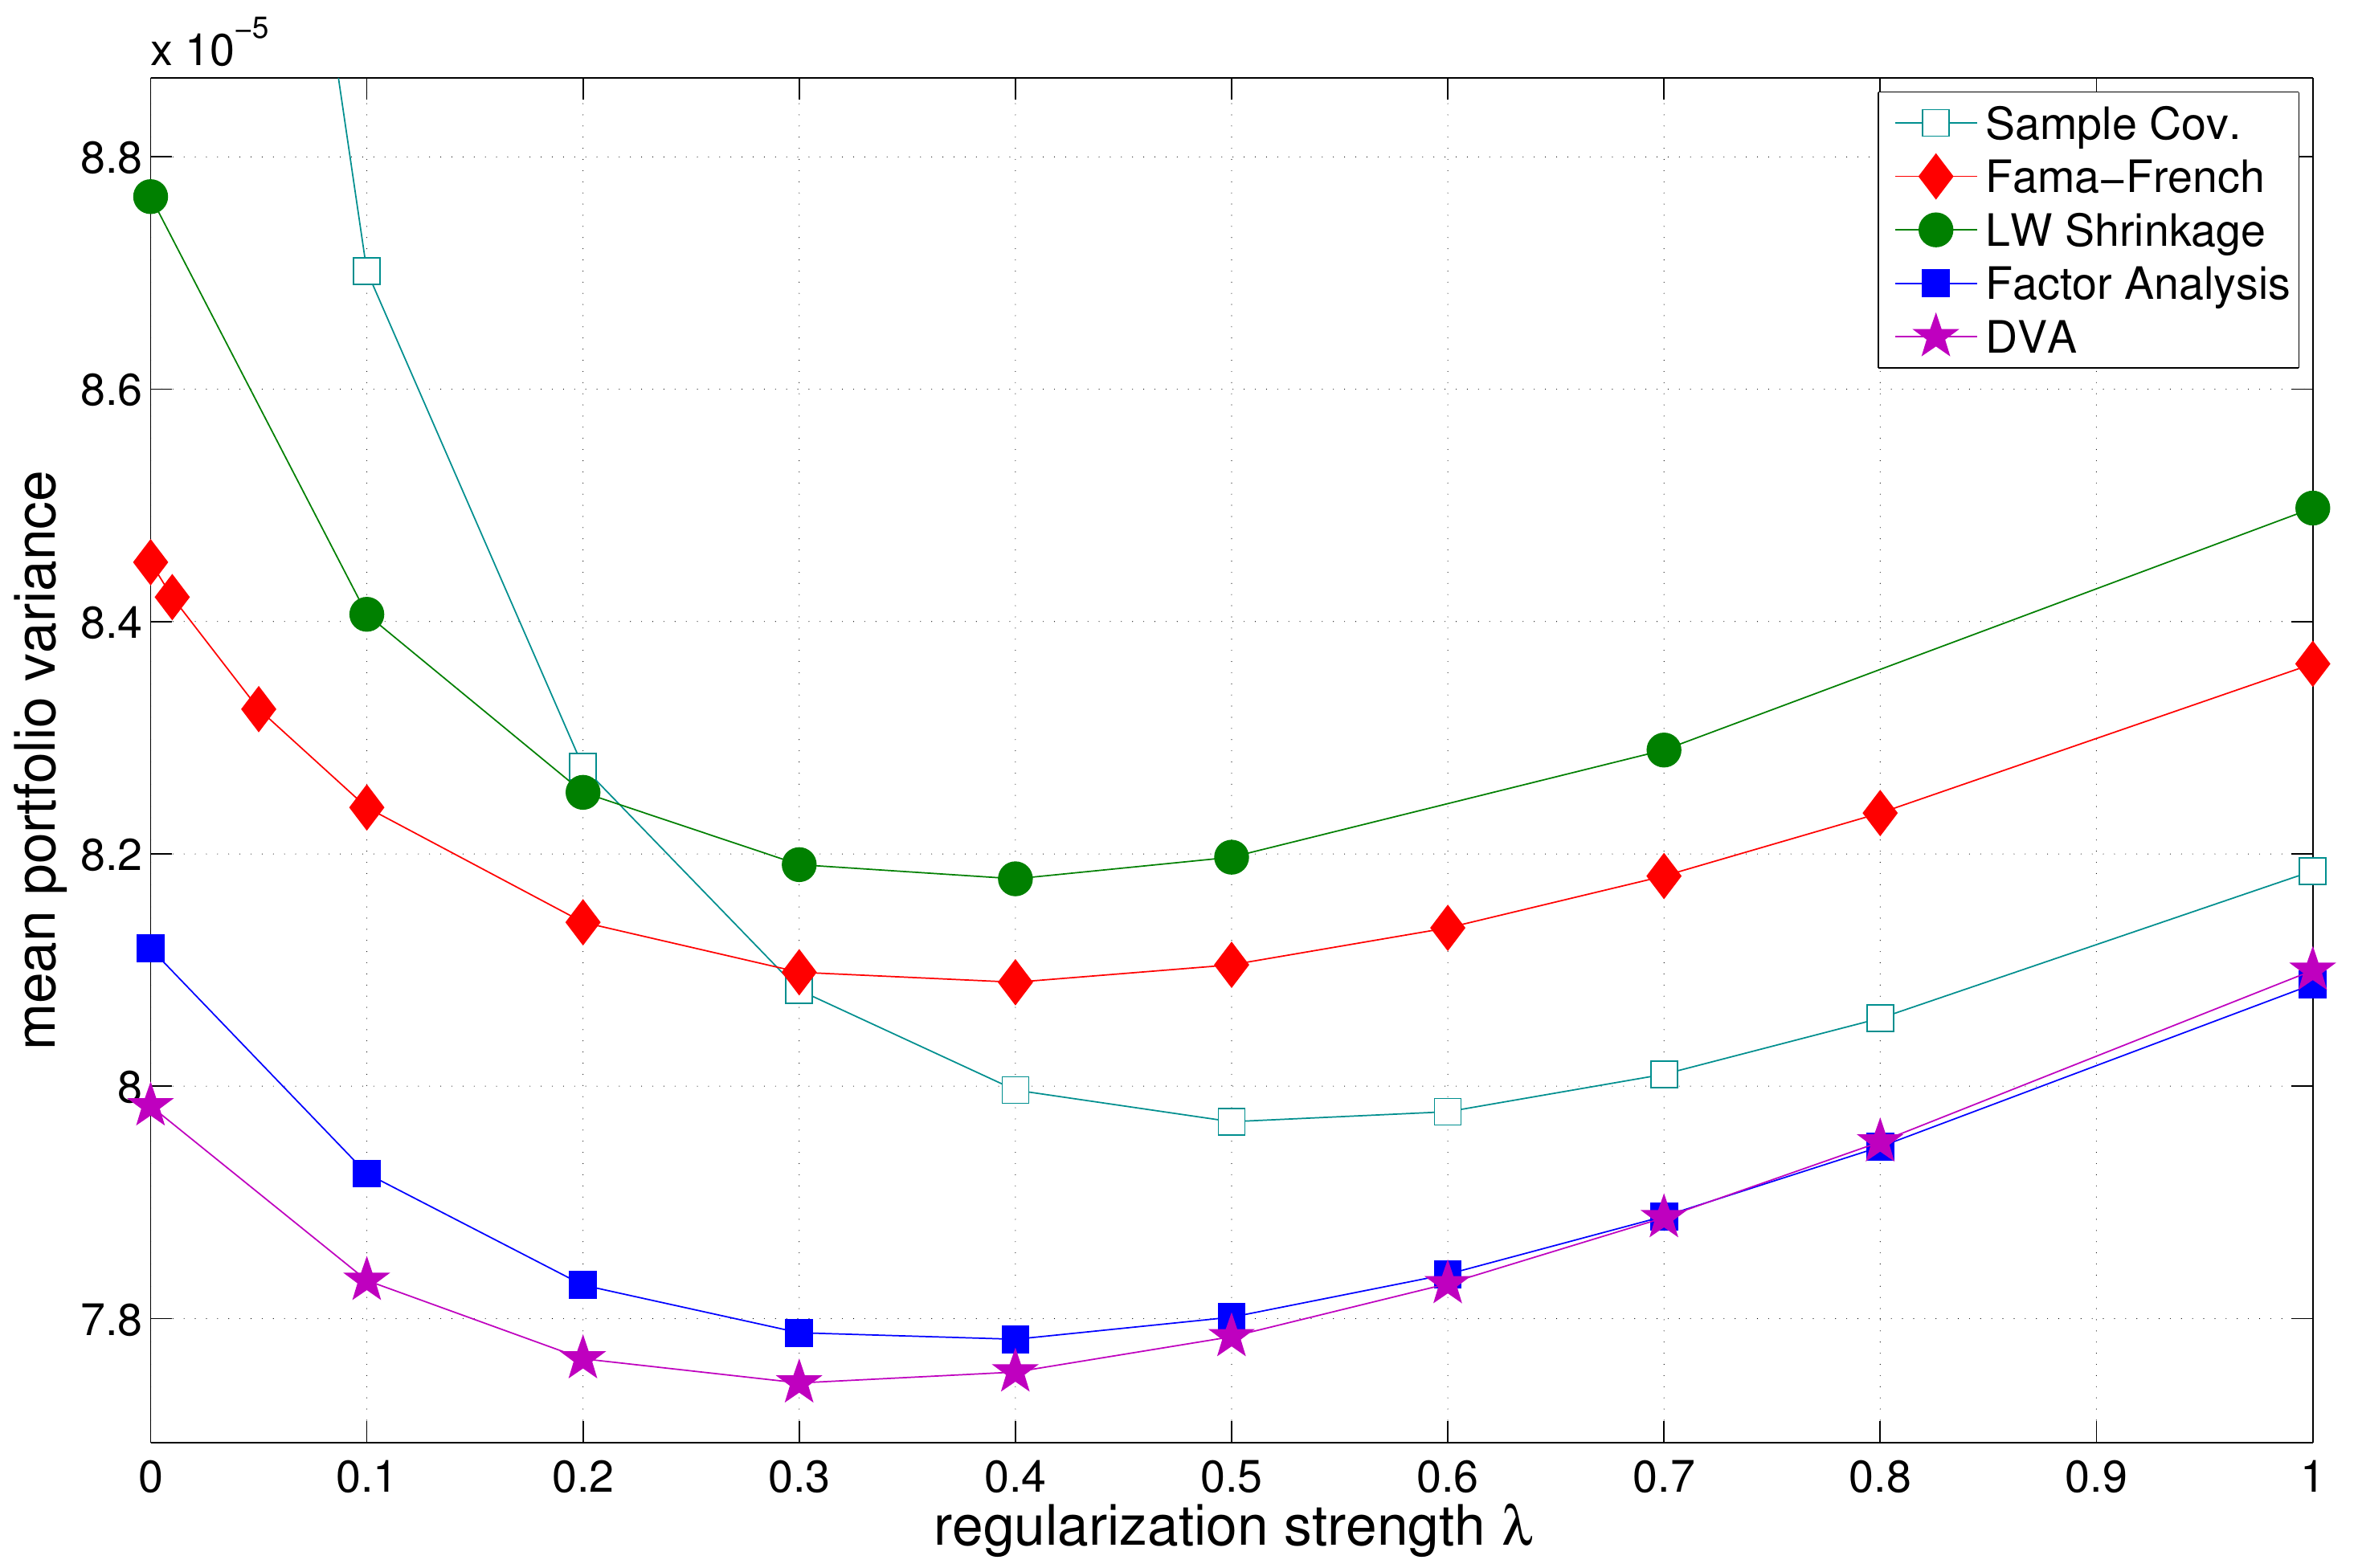}
\caption{variance of optimized portfolios. US market sample~b}
 \label{fig:UScv_reg}
\end{center}
\end{figure}

\begin{figure} 
\begin{center}
\includegraphics[width=.85\textwidth]{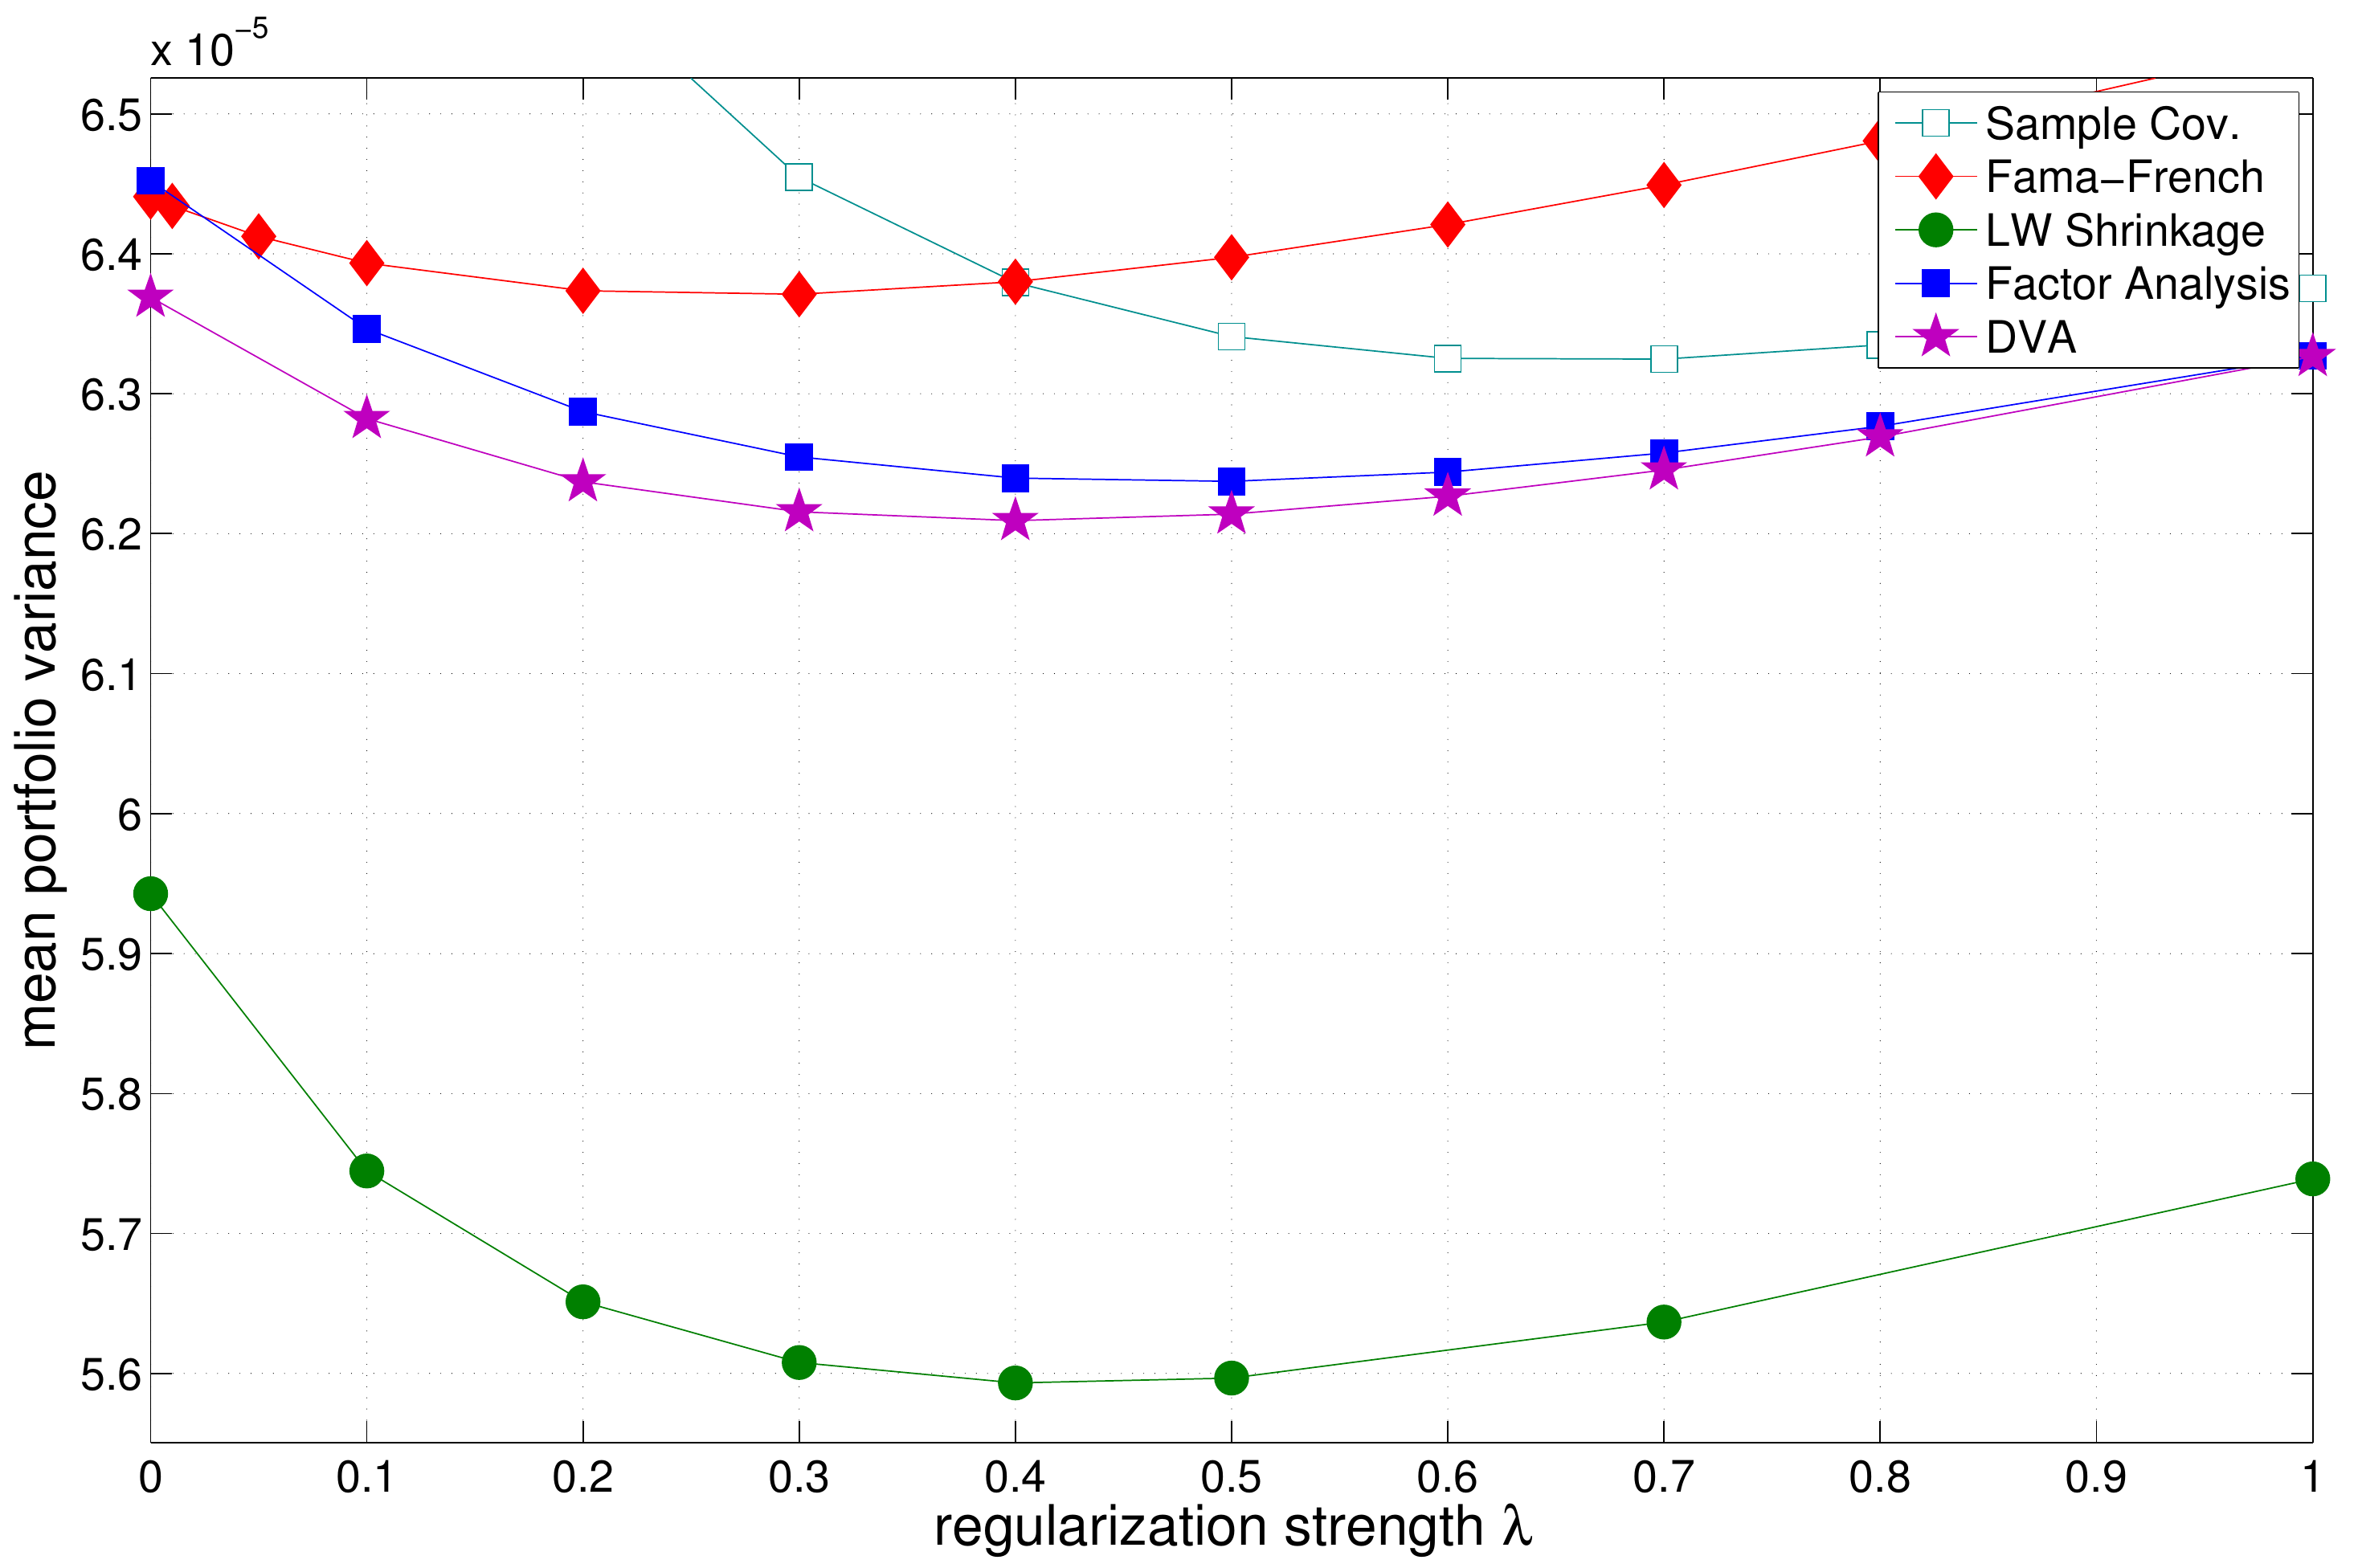}
\caption{variance of optimized portfolios. EU market sample~a}
 \label{fig:EUbv_reg}
\end{center}
\end{figure}

\begin{figure} 
\begin{center}
\includegraphics[width=.85\textwidth]{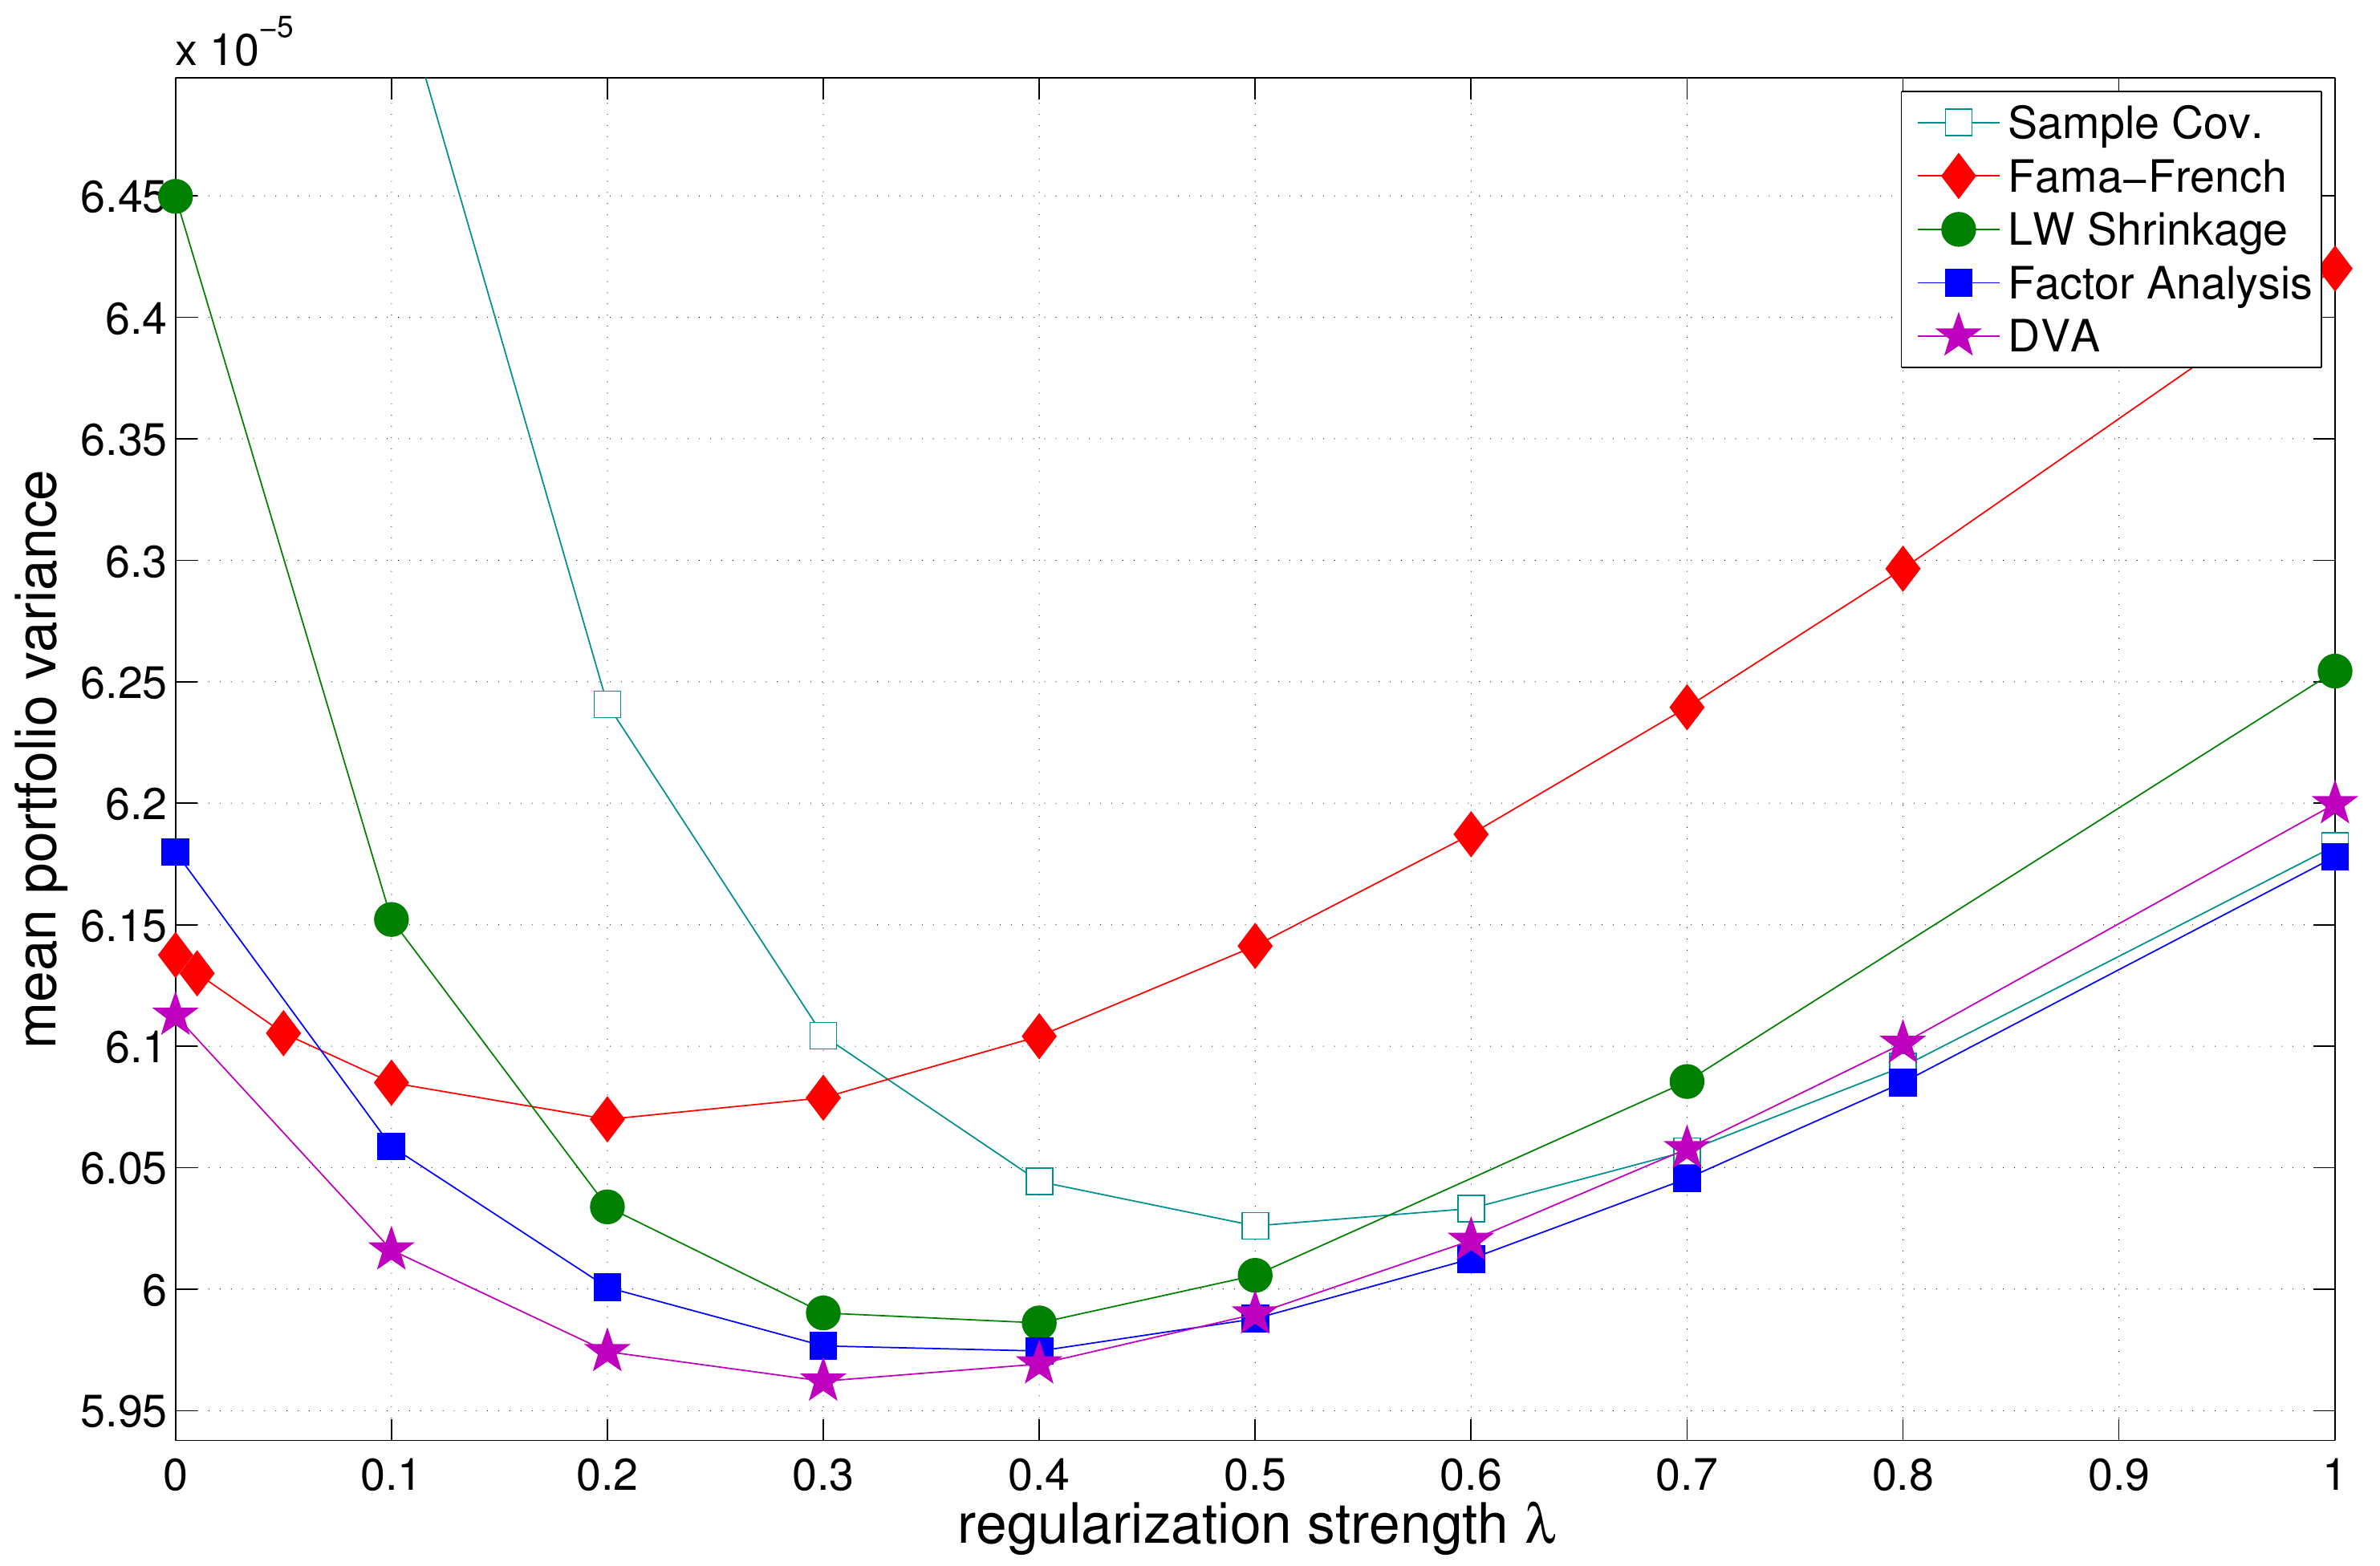}
\caption{variance of optimized portfolios. EU market sample~b}
 \label{fig:EUcv_reg}
\end{center}
\end{figure}

\begin{figure} 
\begin{center}
\includegraphics[width=.85\textwidth]{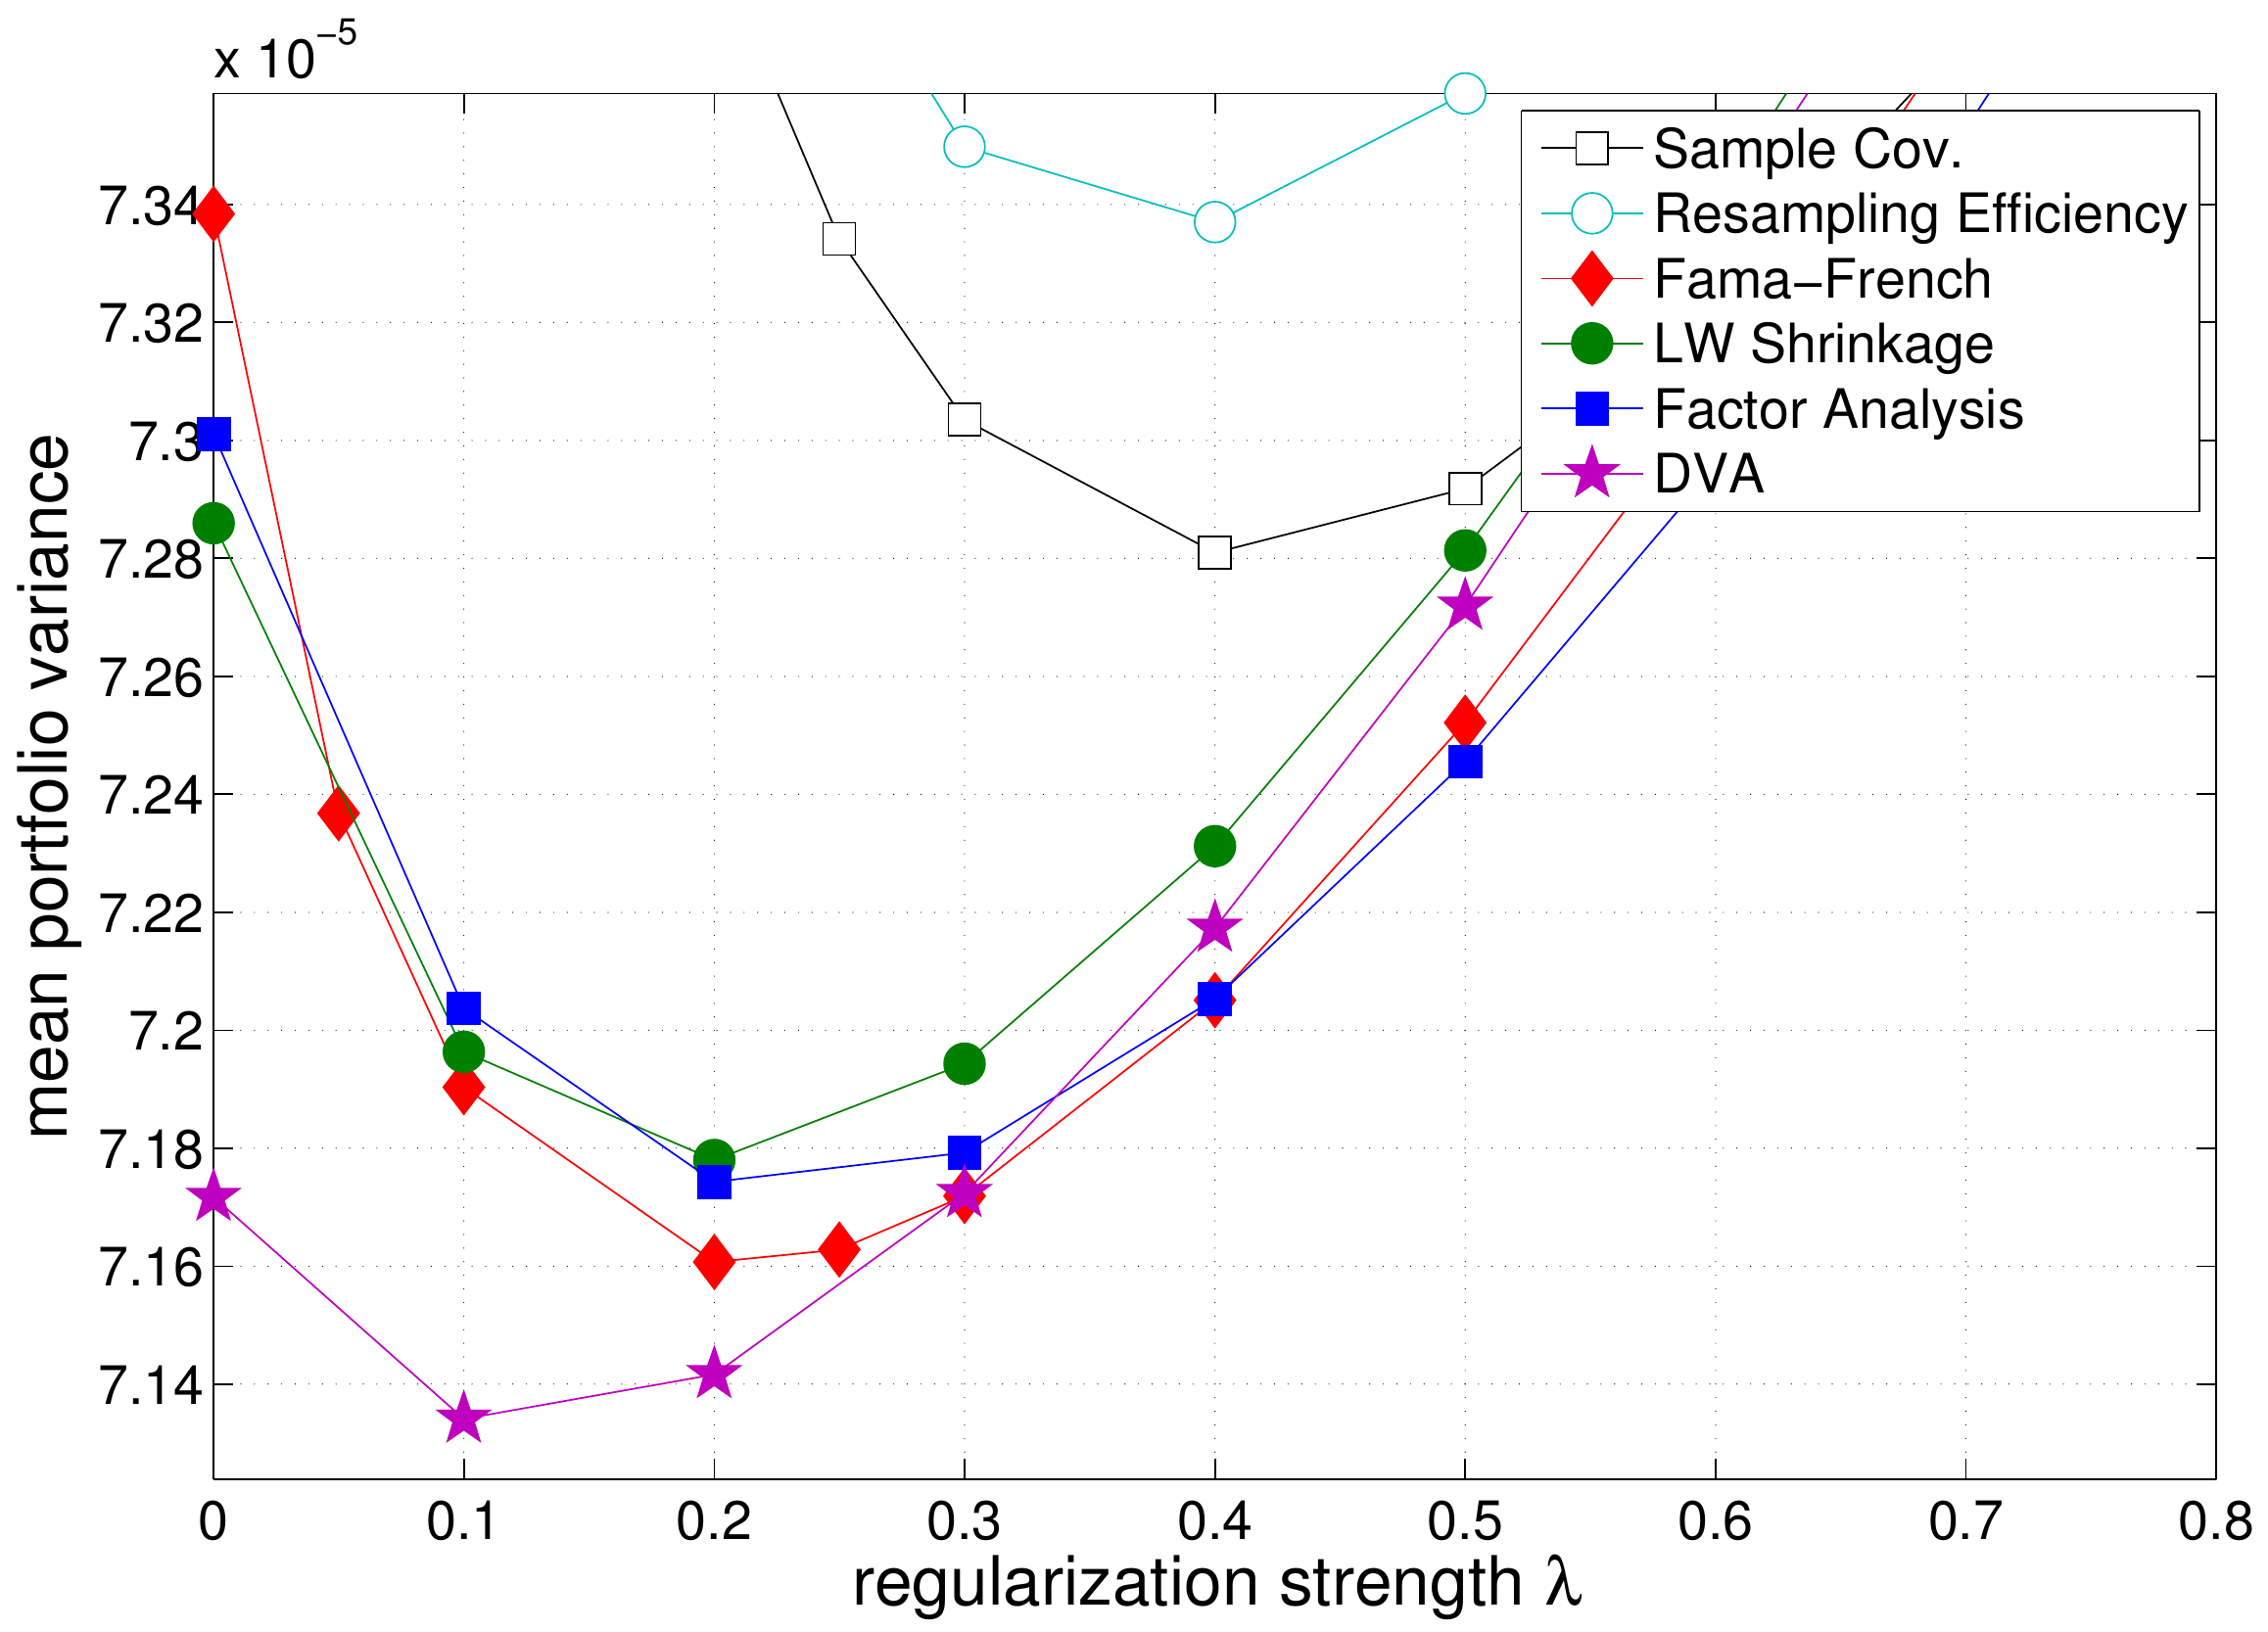}
\caption{variance of optimized portfolios. HK market}
 \label{fig:HKv_reg}
\end{center}
\end{figure}
